# Supplementary material for: An agent design with goal reaching guarantees for enhancement of learning
Source: arXiv:2405.18118 source file (2024-08-21)
Supplement: Supplementary file 1 [file code_appendix.pdf]

# Overview

August 12, 2024

This readme is for the source code for the paper “*An Agent Design with Goal Reaching Guarantees for Enhancement of Learning*”.

The full appendix is located in the file **Appendix.pdf**.

## 1 Installation

### 1.1 Setup Python Virtual Environment

Note that this project requires **Python version 3.10**.

Before running the experiments from the source, it is recommended to set up a virtual environment to isolate the project dependencies. Here’s how to do it:

1. **Install virtualenv if you haven’t got it installed:**

```
pip install virtualenv
```

2. **Create a virtual environment:**

Navigate to the root of the repo and run:

```
virtualenv venv
```

3. **Activate the virtual environment:**

```
source venv/bin/activate
```

### 1.2 Quick start

Once the virtual environment is activated, run the experiments using the following steps:

1. Install the package:

```
sudo apt update
sudo apt install -y libgeos-dev libqt5x11extras5 def
pip install -e .
```

2. Change to the `presets` directory:

```
cd presets
```

3. Run the `reproduce.py` script with the necessary parameters:

```
python reproduce.py --agent={NAME_OF_THE_AGENT} --sy
```

Replace `{NAME_OF_THE_AGENT}` and `{NAME_OF_THE_SYSTEM}` with the corresponding short names from the lists below. For instance:

```
python reproduce.py --agent=calf --env=pendulum
```

4. Navigate to `goalagent/src/code_data/plots/calf_pendulum` to observe the respective learning curve and selected observations from this run.

## 2 Abbreviations

### 2.0.1 Environments

- `--env=inverted_pendulum` for the inverted pendulum
- `--env=pendulum` for the pendulum
- `--env=3wrobot_kin` for the three-wheel robot
- `--env=2tank` for the two-tank system
- `--env=lunar_lander` for the lunar lander
- `--env=omnibot` for the omnibot (kinematic point)

### 2.0.2 Agents

- `--agent=calf` for **our agent**
- `--agent=nominal` for  $\pi_0$
- `--agent=ppo` for Proximal Policy Optimization (PPO)
- `--agent=sdpg` for Vanilla Policy Gradient (VPG)
- `--agent=ddpg` for Deep Deterministic Policy Gradient (DDPG)
- `--agent=reinforce` for REINFORCE
- `--agent=sac` for Soft Actor Critic (SAC)
- `--agent=td3` for Twin-Delayed DDPG (TD3)

## 3 Repo structure

### 3.0.1 `./reproduce.py`

This Python script executes the corresponding bash script to replicate experiments.

### 3.0.2 `./bash`

Within this subdirectory, you can find all the bash scripts intended for running a specific pair agent-environment. You may also override seeds or any hyperparameter here to obtain another set of runs.

### 3.0.3 `presets/validate.py`

A Python script designed for validation purposes. It runs the associated bash script and asserts that the computed total costs match the expected values.

### 3.0.4 Experiment Management Procedures

- **exman:** The 'exman' folder encapsulates the procedures necessary for the handling of experiments.
  - **exman/export.sh:** This script is responsible for exporting all experimental data into an SQLite database, thus ensuring data persistence and easy retrieval.
  - **exman/save\_plot\_data.ipynb:** A Jupyter notebook dedicated to saving the raw data that will be utilized for generating the final plots.
  - **exman/table\_and\_plots.ipynb:** This notebook is tasked with creating the final graphs and tables that are included in the research paper.

### 3.0.5 Comments on Internal Logic of the Repo

**Main script:** Every time you launch `reproduce.py` it will search and launch a respective bash script responsible for a specific agent-environment pair.

**Our agent:** Core logic of our agent is implemented in modules presented in `./goalagent/calf` folder.

### 3.0.6 Hardware and Software Requirements

### 3.0.7 System Configuration

All experiments were conducted on the following machine:

- Operating system: Ubuntu 24.04 LTS
- GPU: 2x GeForce RTX 3090

- CPU: AMD Ryzen Threadripper 3990X 64-Core Processor
- RAM: 128 GB

### **3.0.8 Minimum System Requirements**

- RAM: 32GB or higher
- CPU Cores: At least 16 logical cores
- Storage space: 250 GB for all experiment data
- GPU: Nvidia GPU with a minimum of 10 GB of memory

### **3.0.9 Software Requirements**

All the instructions for preparing the project for running can be found in the section above.

### **3.0.10 Python Dependencies**

All necessary Python dependencies are listed in the `pyproject.toml` file.

### **3.0.11 Non-Python Dependencies**

Non-Python Dependencies can be installed using the following command:

```
sudo apt install -y libgeos-dev libqt5x11extras5 default-jre
```
